# Supplementary material for: Discourse-Aware Neural Extractive Text Summarization
Source: arXiv:1910.14142 source file (2020-04-25)
Supplement: Supplementary file 1 [file sec_9appendix.tex]

\section*{Appendix}
% \subsection{Derivation of Dependency-based Discourse Tree}

% current approach
% problem with current approach
% what we do
% examples

%  Here we give a brief example: [[[Van der Sloot,]$_{\text{N}}$ [handcuffed and wearing a protective vest,]$_{\text{N}}$ ]$_{\text{N}}$ [[was escorted through a news conference]$_{\text{N}}$ [held by Peruvian authorities Saturday.]$_{\text{N}}$]$_{\text{N}}$]$_{\text{N}}$. We use nested paranthesis to denote the parent-child relation. There is an issue that there is no dependencies between `[Van der Sloot,]$_{\text{N}}$', which is the head of `[[Van ...  vest,]$_{\text{N}}$ ]$_{\text{N}}$', and [was escorted through a news conference]$_{\text{N}}$, which is the head of `[[was escorted ... Saturday.]$_{\text{N}}$]$_{\text{N}}$'. Apparently `was escorted through a news conference' is not a standalone grammatical sentence. 
%  \cite{Durrett_Learning_2016} proposed to check if the discourse relation is \textit{SAME\_UNIT} to identify this case which means you have to predict `Van der Sloot' and `was $\cdots$ conference' simultaneously. The problem behind is the annotation agreement is not high enough so \textit{SAME\_UNIT} can be mis-identified. Besides we don't always need to keep both discourse units with \textit{SAME\_UNIT} relations. The example can be `[Jason went to the market,]$_{\text{N}}$ [and John is a server.]$_{\text{N}}$. In this case keeping either of the EDU is grammatically correct. '
 
 \subsection{Visualization of Constructed Graphs $\mathcal{G}_{C}$ \& $\mathcal{G}_{R}$  }
 We show more examples of the constructed Corefeerence Graph $\mathcal{G}_{C}$ and RST Graph $\mathcal{G}_{R}$. 
 
 \input{fig_graph_vis_more.tex}
